# Supplementary material for: Doubly Enhanced Third Harmonic Generation in Metal-Based Silicon Nanodisks
Source: arXiv:1912.11680 source file (2019-12-25)
Supplement: Supplementary file 1 [file Supporting_information_Doubly_enhanced_silicon_THG_YJ_2019Christmas.pdf]

# Supporting information

## Doubly Enhanced Third Harmonic Generation in Metal-Based Silicon Nanodisks

Jin Yao,† Na Liu,† Guoxiong Cai,*,† and Qing Huo Liu*,‡

†*Institute of Electromagnetics and Acoustics, and Fujian Provincial Key Laboratory of Electromagnetic Wave Science and Detection Technology, Xiamen University, Xiamen 361005, China*

‡*Department of Electrical and Computer Engineering, Duke University, Durham, North Carolina 27708, USA*

E-mail: gxcai8303@xmu.edu.cn; qhliu@duke.edu

## Choose of pulse width and its influence on THG efficiency

In the time domain response, the cavity rise-time, representing the time taken for a resonance to grow into the steady state, is required to be considered.[S1] Herein, doubly enhanced EDR is selected for investigation. Its cavity rise-time can be calculated by[S2] $\tau_c = Q\lambda_0/c = 1.44$ ps, where $Q = 280$ is the quality factor of the resonance, $\lambda_0$ is the resonant wavelength and $c$ is the speed of light. The $x$-polarized time-harmonic plane wave with the angular frequency $\omega = \frac{2\pi c}{\lambda_0}$, defined by $E_x = E_{inc} \cos(\omega t - k_0 z)$, is thus illuminated normally on the proposed metal-dielectric nanostructures. The peak amplitude of electric field is $E_{inc} = 1.504\times10^7$ V/m, corresponding to an input intensity 0.03 GW/cm$^2$. Figure S1a gives the normalized time domain responses of the incidence and the average electric field enhancement $|E_{avg}/E_{inc}|$ inside the silicon nanodisk at resonant wavelength $\lambda_0 = 1540$ nm. It can be seen that the electric field inside silicon gradually rises and reaches a stable value after time $t = 1.45$ ps, which is basically consistent with the calculated cavity rise-time.

According to the analysis above, the chosen time domain pulse should be at least wider than the cavity rise-time to obtain a completely excited system. Herein, the incidence is adjusted to a Gaussian pulsed plane wave with $E_x = E_{inc}\cos(\omega t - k_0 z)e^{-(\frac{t-t_0}{\Delta t})^2}$, and the dependence of the pulse width $\Delta t$ on the THG efficiency is thus plotted in Figure S1b. With the pulse width

increasing, the THG efficiency is raised and nearly remains constant after $\Delta t$ = 2 ps. Therefore, as a guidance in the practical operation, the pulse width $\Delta t$ > 2 ps is required to be chosen to ensure an efficient resonant excitation and thus the intact nonlinear response.

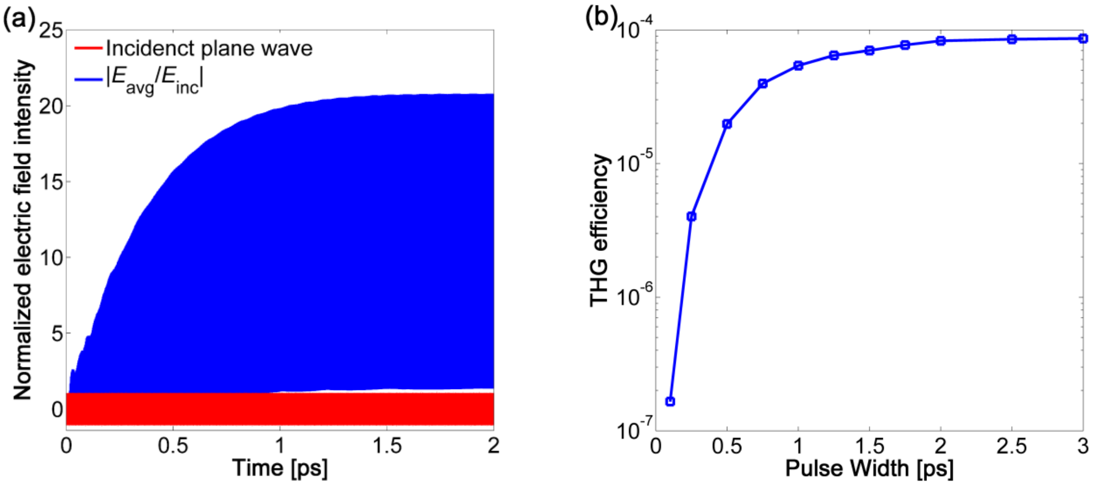


Figure S1: (a) Normalized time domain responses of the incidence and the average electric field enhancement $|E_{avg}/E_{inc}|$ inside the silicon nanodisk at resonant wavelength $\lambda_0$ = 1540 nm. (b) Dependence of the pulse width $\Delta t$ on the THG efficiency.

## References


[S1] Yang, Y.; Wang, W.; Boulesbaa, A.; Kravchenko, I. I.; Briggs, D. P.; Puretzky, A.; Geohegan, D.; Valentine, J. Nonlinear Fano-Resonant Dielectric Metasurfaces. *Nano Lett.* **2015**, *15* (11), 7388-7393.

[S2] Huang, Z.; Baron, A.; Larouche, S.; Argyropoulos, C.; Smith, D. R. Optical bistability with film-coupled metasurfaces. *Opt. Lett.* **2015**, *40* (23), 5638-5641.
